# Supplementary material for: Globally Convergent Policy Search over Dynamic Filters for Output Estimation
Source: arXiv:2202.11659 source file (2022-02-25)
Supplement: Supplementary file 2 [file cvx_fact.tex]

%!TEX root = ../main.tex
