# Supplementary material for: Globally Convergent Policy Search over Dynamic Filters for Output Estimation
Source: arXiv:2202.11659 source file (2022-02-25)
Supplement: Supplementary file 3 [file appendix.tex]

\section{Technical Lemmas}

\begin{lemma}[Schur Complement Theorem]
\label{lemma:schur_complement}
Let $A \succ 0$ and let $C \in \mathcal{S}^n$. Then, the matrix $M$ defined as
\begin{align*}
	M = \begin{bmatrix}
		A & B \\ 
		B^\top & C
	\end{bmatrix}
\end{align*}
is positive (semi)definite if and only if $C - B^\top A^{-1}B$ is positive (semi)definite. Similarly, if C is positive definite, then $M$ is positive definite if and only if $A - BC^{-1}B^\top$ is positive definite.
\end{lemma}
